# Supplementary material for: QuanTemp: A real-world open-domain benchmark for fact-checking numerical claims
Source: arXiv:2403.17169 source file (2024-05-01)
Supplement: Supplementary file 1 [file supplementary.tex]

\subsection{Topical Point of view}

In this point-of-view, numerical fact-checking queries specifically involve verifying the accuracy of numerical information presented in a claim or statement. 
This verification is topical -- statistical, geographical, economic,economic, or scientific.  
Numerical fact-checking can be seen as a subset of QA where the answer is not just a number or explanation but a validation of a numerical claim. 
Numerical fact-checking queries can typically be classified into several types:

\begin{itemize}
  \item \textbf{Statistical Data Verification:} Questions that verify statistical claims by referencing authoritative data sources. 
  Example: Checking if a statement like ``The unemployment rate dropped to 3.5\% last month'' aligns with official labor statistics.

  \item \textbf{Historical Data Validation:} Queries that validate historical numbers or data points.
  Example: Confirming the accuracy of ``The company's revenue was \$10 million in 2005.''

  \item \textbf{Geographical Data Authentication:} Inquiries that check numerical claims related to geography.
  Example: Verifying whether ``The Amazon River is over 7000 kilometers long.''

  \item \textbf{Scientific Measurement Confirmation:} Queries that confirm measurements reported in scientific research.
  Example: Fact-checking a claim like ``The medicine has a 90\% efficacy rate.''

  \item \textbf{Checking Economic Data:} Questions that corroborate economic figures presented in reports or news.
  Example: Examining the claim ``Inflation rates have increased by 2\% in the first quarter.''
  
  \item \textbf{Public Record Consistency Checks:} Queries that ensure consistency with public records. \textcolor{teal}{Maybe this overlaps with Statistical Data Verification}.
  Example: Checking if ``The city's population is 1.2 million according to the latest census.'' 

\end{itemize}
