# Supplementary material for: QuanTemp: A real-world open-domain benchmark for fact-checking numerical claims
Source: arXiv:2403.17169 source file (2024-05-01)
Supplement: Supplementary file 2 [file 08_appendix.tex]

\appendix

\section{Detailed claim collection process}
